# Supplementary material for: A Mixing Time Lower Bound for a Simplified Version of BART
Source: arXiv:2210.09352 source file (2022-10-17)
Supplement: Supplementary file 1 [file _supp.tex]

\appendix

\counterwithin{figure}{section}
\counterwithin{table}{section}

\newpage
\onecolumn

\begin{center}
    \Huge
    Supplement 
\end{center}
\label{sec:supp}

\section{\methods run-time analysis}
\label{sec:runtime_supp}

\begin{proposition}
    The run time complexity for \method~to grow a model with $m$ splits in total is $O(dm^2n^2)$, where $d$ the number of features, and $n$ the number of samples.
\end{proposition}

\begin{proof}
    Each iteration of the outer loop adds exactly one split, so it suffices to bound the running time for each iteration, where it is clear that the cost is dominated by the operation $\texttt{split}$ in~\cref{alg:method} line 9, which takes $O(n^2 d)$, since there are at most $n d$ possible splits, and it takes $O(n)$ time to compute the impurity decrease for each of these.
    Consider iteration $s$, in which we have a \method~model $f$ with $s$ splits. 
    Suppose $f$ comprises $k$ trees in total, with tree $i$ having $s_i$ splits, and so that $s = s_1 + \ldots + s_k$.
    The total number of potential splits is equal to $l+1$, where $l$ is the total number of leaves in the model.
    The number of leaves on each tree is $s_i + 1$, so the total number of leaves in $f$ is
    $$
    l = \sum_{i=1}^k (s_i+1) = s + k.
    $$
    Since each tree has at least one split, we have $k \leq s$, so that the number of potential splits is at most $2s+1$
    The total time complexity is therefore
    $$
    \sum_{s=1}^m (2s+1) \cdot O(n^2 d) = O(m^2n^2d).
    $$
\end{proof}

\section{Simulations}

\label{sec:sims_supp}

\subsection{Error rate for \methods for two generative models.}

%In the follWe simulated data via a sparse sum of squares model $y = \sum_{j=1}^{20} x^2_j + \epsilon$  with $\bx \sim \text{Unif}\paren*{[0,1]^{50}}$, and $\epsilon \sim N(0,0.01)$. 

\begin{figure}[H]
    \centering
    \begin{tabular}{cc}
         (A) Sum-of-squares model & (B) Linear model \\
         \includegraphics[width=0.45\columnwidth]{figs/err_rate_1_sum_of_squares.pdf} &  \includegraphics[width=0.45\columnwidth]{figs/err_rate_0_linear_model.pdf}
    \end{tabular}
    \caption{\methods test error rate is faster than CART and random forest.
    In both (A) and (B), the generative model for $X$ is uniform with 50 features.
    Noise is Gaussian with mean zero and standard deviation 0.1 for training but no noise for testing.
    \textit{(A)}
    $Y$ is generated as sum of squares of $X_i$ for sparsity 20 with coefficient 1.
    Averaged over 4 runs.
    \textit{(B)} 
    $Y$ is generated from a linear model where $X_i$ for sparsity 10 with coefficient 1.
    Averaged over 4 runs.
    }
    \label{fig:err_rate_supp}
\end{figure}

\subsection{Comparison of \methods performance with those of other algorithms over more generative models}

\label{subsec:more_sims_supp}

We compare the prediction performance of \methods against that of four other algorithms: CART, RF, XGBoost, and penalized iteratively reweighted least squares (PIRLS) on the log-likelihood of a generative additive model.
We simulated data via $y = f(\bx) + \epsilon$  with $\bx \sim \text{Unif}\paren*{[0,1]^{50}}$, and $\epsilon \sim N(0,0.01)$, where $f$ is one of the four regression functions:
\begin{enumerate}
    \item[(A) Linear model:] $f(\bx) = \sum_{i=1}^{20} x_i$
    \item[(B) Single Boolean interaction model:] $f(\bx) = \prod_{i=1}^8\indicator\braces*{x_i > 0.1}$
    \item[(C) Sum of polynomial interactions model:] $f(\bx) = \sum_{i=0}^4 x_{3i+1}x_{3i+2}x_{3i+3}$
    \item[(B) Sum of Boolean interactions model:] $f(\bx) = \sum_{i=0}^4\prod_{j=1}^3\indicator\braces*{x_{3i+j} > 0.5}$
\end{enumerate}

We ran \methods with a minimum impurity decrease threshold of $5\sigma^2$.
We used the implementation of PIRLS in \texttt{pygam} \cite{daniel_serven_2018_1476122}, with 20 splines term for each feature.
All other algorithms were fitted using default settings, except that we set \texttt{min\_samples\_leaf=5} in CART.
We computed the noiseless test MSE for all five algorithms on each of the generative models for a range of sample sizes $n$, averaging the results over 10 runs.

The results, plotted in \cref{fig:more_sims_supp}, show that while all other models suffer from weaknesses (PIRLS performs poorly whenever there are interactions present, i.e. for (B), (C) and (D), and tree-based methods perform poorly when there is additive structure in (A)),
\methods is able to adapt well to all scenarios, usually outperforming all other methods in moderate sample sizes.

\begin{figure}[H]
    \centering
    \begin{tabular}{cc}
         (A) Linear model & (B) Single interaction model \\
         \includegraphics[width=0.45\columnwidth]{figs/linear_error_curves.png} &  \includegraphics[width=0.45\columnwidth]{figs/single_interaction_error_curves.png} \\
         (C) Sum of polynomial interactions model & (D) Sum of Boolean interactions model \\
         \includegraphics[width=0.45\columnwidth]{figs/poly_error_curves.png} &  \includegraphics[width=0.45\columnwidth]{figs/LSS_error_curves.png}
    \end{tabular}
    \caption{\methods is able to adapt to generative models, handling both additive structure and interactions gracefully.
    In both (A) and (B), the generative model for $X$ is uniform with 50 features.
    Noise is Gaussian with mean zero and standard deviation 0.1 for training but no noise for testing.
    \textit{(A)}
    $Y$ is generated as linear model with sparsity 20 and coefficient 1.
    \textit{(B)} 
    $Y$ is generated from a single Boolean interaction model of order 8.
    \textit{(C)} 
    $Y$ is generated from a sum of 5 three-way polynomial interactions.
    \textit{(D)} 
    $Y$ is generated from a sum of 5 three-way Boolean interactions.
    All results are averaged over 10 runs.
    }
    \label{fig:more_sims_supp}
\end{figure}

\section{Data details}
\label{sec:data_supp}

\begin{table}[H]
    \footnotesize%\small
    \centering
    \input{figs/data_classification_full}
    \caption{Classification datasets (extended).}
    \label{tab:data_classification_full}
\end{table}

\begin{table}[H]
    \footnotesize%\small
    \centering
    \input{figs/data_regr_full}
    \caption{Regression datasets (extended).}
    \label{tab:data_regr_full}
\end{table}

\section{Experiment results}

\begin{figure}[H]
    \centering
    \includegraphics[width=0.5\columnwidth]{figs/num_trees.pdf}
    \caption{Number of trees learned as a function of the total number of rules in \methods for different classification datasets.}
    \label{fig:num_trees}
\end{figure}

\begin{figure}[H]
    \centering
    \includegraphics[width=0.5\columnwidth]{figs/repeated_splits_full.pdf}
    \caption{Fraction of repeated splits for all datasets. Corresponds to \cref{fig:repeated_subtrees}.}
    \label{fig:repeated_splits_full}
\end{figure}

\section{Proof details for \cref{sec:theory}}
\label{sec:theory_supp}

\subsection{Proof of \cref{thm:generalization_main}}

\begin{proof}[Proof of \cref{thm:generalization_main}]
    We may assume WLOG that $\E_{\pi_k}\braces*{f_k} = 0$ for each $k$.
    We first define the feature mappings $\Psi_k$ for each set of indices $I_k$ and concatenate them to form our feature map $\Psi$.
    To define $\Psi_k$, consider a tree $\tree_k$ that partitions $[0,1]^{d_k}$ into cubes of side length $h_k$, where $h_k$ is a parameter to be determined later.
    Let $p_k$ denote the number of internal nodes in $\tree_k$.
    Let $g_k$ be defined by 
    \begin{equation*}
        g_k(\bx_{I_k}) \coloneqq \E\braces*{f_k(\bx_{I_k}')~|~\bx_{I_k}' \in \node_k(\bx_{I_k})}
    \end{equation*}
    where $\node_k(\bx_{I_k})$ is the leaf in $\tree_k$ containing $\bx_{I_k}$, and $\bx_{I_k}'$ an independent copy of $\bx_{I_k}$.
    Set
    \begin{equation} \label{eq:formula_for_theta_star}
        \btheta^*(\node) \coloneqq \frac{\sqrt{N(\node_L)N(\node_R)}}{N(\node)}\paren*{\E\braces*{y~|~\node_L} - \E\braces*{y~|~\node_R}},
    \end{equation}
    for each node $\node$ to form a vector $\btheta^* \in \R^p$, where $p = \sum_{k=1}^K p_k$.
    One can check that
    $$
    g_k(\bx_{I_k}) = \btheta_{I_k}^{*T}\Phi_k(\bx_{I_k}).
    $$
    Now define
    $$
    g(\bx) = \sum_{k=1}^K g_k(\bx_{I_k}) = \btheta^T\Phi(\bx).
    $$
    %By construction, the coordinates of $\Phi_k(\bx_{I_k})$ are orthogonal to each other as random variables, and because of the independence of $\bx_{I_j}$ and $\bx_{I_k}$ for $j \neq k$, we see also that the coordinates of $\Phi(\bx)$ are also orthogonal to each other.
    For any event $\mathcal{E}$, we may apply Cauchy-Schwarz to get
    \begin{equation} \label{eq:Cauchy_Schwarz}
        \E_{\data, \bx \sim \pi} \braces*{\paren*{\tilde f(\bx) - f(\bx)}^2\indicator\braces*{\mathcal{E}^c}} 
        \leq 2\E\braces*{\paren*{f(\bx)- g(\bx)}^2} + 2\E\braces*{\paren*{g(\bx)- \tilde f(\bx)}^2\indicator\braces*{\mathcal{E}^c}}.
    \end{equation}
    By independence, and the fact that $\E\braces*{g_k(\bx_{I_k})} = 0$ for each $k$, we can decompose the first term as
    \begin{equation*}
        \E\braces*{\paren*{f(\bx)- g(\bx)}^2} = \sum_{k=1}^K \E\braces*{\paren*{f_k(\bx)- g_k(\bx)}^2}.
    \end{equation*}
    Meanwhile, note that we have the equation
    $$
    y = \btheta^{*T}\Psi(\bx) + \eta + \epsilon
    $$
    where $\eta \coloneqq f(\bx) - g(\bx)$ satisfies
    \begin{align*}
        \E\braces*{\eta~|~\Psi(\bx)}
        & = \E\braces*{\sum_{k=1}^K \paren*{f_k(\bx_{I_k}) - g_k(\bx_{I_k})}~|~\Psi(\bx)} \\
        & = \sum_{k=1}^K\E\braces*{ f_k(\bx_{I_k}) - g_k(\bx_{I_k})~|~\Psi_k(\bx_{I_k})} \\
        & = 0.
    \end{align*}
    As such, we may apply Theorem \ref{thm:generalization_lin_reg} with the event $\mathcal E$ given in the statement of the theorem to get
    \begin{align*}
        \E\braces*{\paren*{g(\bx)- \tilde f(\bx)}^2\indicator\braces*{\mathcal E ^c}} \leq 2\paren*{\frac{p\sigma^2}{n+1} + 2\E\braces*{\paren*{f(\bx)- g(\bx)}^2}}.
    \end{align*}
        \begin{equation}
        \E_{\data,\bx}\braces*{\paren*{\bx^T\paren*{\hat\btheta_{n} - \btheta}}^2\indicator\braces*{\mathcal E ^c}}
        \leq 2\paren*{\frac{p\sigma_\epsilon^2}{n+1} + 2\sigma_\eta^2}.
    \end{equation}
    Plugging this into \eqref{eq:Cauchy_Schwarz}, we get
    \begin{align} \label{eq:continuation_of_CS}
        \E_{\data, \bx \sim \pi} \braces*{\paren*{\tilde f(\bx) - f(\bx)}^2\indicator\braces*{\mathcal{E}^c}} 
        & \leq 10\sum_{k=1}^K \E\braces*{\paren*{f_k(\bx_{I_k})- g_k(\bx_{I_k})}^2} + \frac{4p\sigma^2}{n+1} \nonumber \\
        & = \sum_{k=1}^K \paren*{10\E\braces*{\paren*{f_k(\bx_{I_k})- g_k(\bx_{I_k})}^2} + \frac{4p_k\sigma^2}{n+1}}.
    \end{align}
    
    We reduce to the case of uniform distribution $\mu$, via the inequality
    $$
    \E_{\pi_k}\braces*{\paren*{f_k(\bx_{I_k})- g_k(\bx_{I_k})}^2} \leq \norm{\pi_k}_\infty\E_\mu\braces*{\paren*{f_k(\bx_{I_k})- g_k(\bx_{I_k})}^2},
    $$
    and from now work with this distribution, dropping the subscript for conciseness.
    Next, observe that
    \begin{equation*}
        \E\braces*{\paren*{f_k(\bx_{I_k})- g_k(\bx_{I_k})}^2} = \E\braces*{\Var\braces*{f_k(\bx_{I_k})~|~\node_k(\bx_{I_k})}}.
    \end{equation*}
    Using Lemma \ref{lem:variance_and_sides}, we have that
    \begin{equation*}
        \Var\braces*{f_k(\bx_{I_k})~|~\node_k(\bx_{I_k})} 
        \leq \frac{\beta_k^2d_k h_k^2}{6}.
    \end{equation*}
    Meanwhile, a volumetric argument gives
    \begin{equation*}
        p_k \leq h_k^{-d_k}.
    \end{equation*}
    We use these to bound each term of \eqref{eq:continuation_of_CS} as
    \begin{equation} \label{eq:continuation_of_CS_pt2}
        10\norm{\pi_k}_\infty\E\braces*{\paren*{f_k(\bx_{I_k})- g_k(\bx_{I_k})}^2} + \frac{4p_k\sigma^2}{n+1} 
        \leq 2\norm{\pi_k}_\infty\beta_k^2d_k h_k^2 + \frac{4h_k^{-d_k}\sigma^2}{n+1}.
    \end{equation}
    Pick
    $$
    h_k = \paren*{\frac{2\sigma^2}{\norm{\pi_k}_\infty\beta_k^2d_k(n+1)}}^{\frac{1}{d_k+2}},
    $$
    which sets both terms on the right hand side to be equal, in which case the right hand of \eqref{eq:continuation_of_CS_pt2} has the value
    \begin{equation*}
        4\paren*{2\norm{\pi_k}_\infty\beta_k^2d_k}^{\frac{d_k}{d_k+2}}\paren*{\frac{\sigma^2}{n+1}}^{\frac{2}{d_k+2}}.
    \end{equation*}
    Summing these quantities up over all $k$ gives the bound \eqref{eq:generalization_bound_theorem}, with the error probability obtained by computing $2p/n$.
\end{proof}

\begin{corollary} \label{cor:sparse_additive}
    Assume a sparse additive model, i.e. in \eqref{eq:additive}, assume $I_k = \braces{k}$ for $k=1,\ldots,K$. Then we have
    $$
    \E_{\data, \bx \sim \pi} \braces*{\paren*{\tilde f(\bx) - f(\bx)}^2\indicator\braces*{\mathcal{E}^c}}
    \leq 8K\max_k \paren*{\norm{\pi_k}_\infty\beta_k^2}^{1/3}\paren*{\frac{\sigma^2}{n}}^{\frac{2}{3}}.
    $$
\end{corollary}

\begin{lemma}[Variance and side lengths] \label{lem:variance_and_sides}
    Let $\uniform$ be the uniform measure on $[0,1]^d$. 
    Let $\cell \subset [0,1]^d$ be a cell. Let $f$ be any differentiable function such that $\norm{\grad f(\bx)}_2^2 \leq \beta^2$.
    Then we have
    \begin{equation} \label{eq:variance_and_sides}
        \Var_\mu\braces*{f(\bx)~|~\bx \in \cell} \leq \frac{\beta^2}{6}\sum_{j=1}^d (b_j-a_j)^2.
    \end{equation}
\end{lemma}

\begin{proof}
    For any $\bx, \bx' \in \cell$, we may write
    $$
    \paren*{f(\bx) - f(\bx')}^2 = \inprod*{\grad f(\bx''),\bx - \bx'}^2 \leq \beta^2 \norm{\bx-\bx'}_2^2.
    $$
    Next, note that
    $$
    \E\braces*{\norm{\bx-\bx'}_2^2~|~\bx,\bx' \in \cell}^2 = \frac{1}{3}\sum_{j=1}^d (b_j-a_j)^2.
    $$
    As such, we have
    \begin{align*}
        \Var_\mu\braces*{f(\bx)~|~\bx \in \cell} & = \frac{1}{2}\E\braces*{\paren*{f(\bx) - f(\bx')}^2~|~ \bx, \bx' \in c\ell} \\
        & \leq \frac{\beta^2}{6}\sum_{j=1}^d (b_j-a_j)^2.
    \end{align*}
\end{proof}

\subsection{Proof of \cref{thm:disentanglement}}

\begin{proof}[Proof of \cref{thm:disentanglement}]
    We prove this by induction on the total number of splits, with the base case being trivial.
    %For any tree component $\hat f_k$ of the model, let $I(\hat f_k)$ denote the index set of features split upon in $\hat f_k$.
    By the induction hypothesis, we may assume WLOG that $\hat f_1$ only has splits on features in $I_1$.
    Consider a candidate split $s$ on a leaf $\node \in \hat f_1$ based on a feature $m \in I_2$.
    Let $\node' = P_1(\node)$. 
    As sets in $\R^d$, we may then write
    \begin{equation} \label{eq:disentanglement_node_formula}
        \node = \node' \times \R^{[d]\backslash I_1},
    \end{equation}
    \begin{equation} \label{eq:disentanglement_node_left_formula}
        \node_L = \node' \times (-\infty, \tau] \times \R^{[d]\backslash I_1\cup \braces{m}},
    \end{equation}
    and
    \begin{equation} \label{eq:disentanglement_node_right_formula}
        \node_R = \node' \times (\tau, \infty) \times \R^{[d]\backslash I_1\cup \braces{m}}.
    \end{equation}
    
    Recall that we work with the residual $r^{(-1)} = f(\bx) - \sum_{k > 1} \hat f_k$.
    Now using the law of total variance, we can rewrite the weighted impurity decrease in a more convenient form:
    \begin{equation} \label{eq:disentanglement_imp_dec}
        \Delta(s,\node, r^{(-1)}) = \frac{\pi(\node_L)\pi(\node_R)}{\pi(\node)} \paren*{\E\braces*{r^{(-1)}~|~\bx \in \node_L} - \E\braces*{r^{(-1)}~|~\bx \in \node_R}}^2.
    \end{equation}
    We may assume WLOG that this quantity is strictly positive.
    By the induction hypothesis, we can divide the set of component trees into two collections, one of which only splits on features in $I_2$, and those which only split on features in $[d]\backslash I_2$.
    Denoting the function associated with the second collection of trees by $g_2$, we observe that
    \begin{equation*}
        \E\braces*{r^{(-1)}~|~\bx \in \node_L} - \E\braces*{r^{(-1)}~|~\bx \in \node_R}
        = \E\braces*{f_2 - g ~|~\bx \in \node_L} - \E\braces*{f_2 - g ~|~\bx \in \node_R}.
    \end{equation*}
    Since $f_2$ and $g$ do not depend on features in $I_1$, we can then further rewrite this quantity as
    \begin{equation} \label{eq:disentanglement_cond_exp}
        \E\braces*{f_2 - g ~|~x_m \leq \tau} - \E\braces*{f_2 - g ~|~x_m > \tau}.
    \end{equation}
    Meanwhile, using \eqref{eq:disentanglement_node_formula}, \eqref{eq:disentanglement_node_left_formula}, and \eqref{eq:disentanglement_node_right_formula}, we may rewrite
    \begin{equation} \label{eq:disentanglement_probs}
        \frac{\pi(\node_L)\pi(\node_R)}{\pi(\node)} = \pi_1(\node')\pi_2(x_m \leq \tau)\pi_2(x_m > \tau).
    \end{equation}
    Plugging \eqref{eq:disentanglement_cond_exp} and \eqref{eq:disentanglement_probs} back into \eqref{eq:disentanglement_imp_dec}, we get
    \begin{equation} \label{eq:disentanglement_imp_dec_smaller}
        \Delta(s,\node, r^{(-1)}) = \pi_1(\node')\pi_2(x_m \leq \tau)\pi_2(x_m > \tau) \paren*{\E\braces*{f_2 - g ~|~x_m \leq \tau} - \E\braces*{f_2 - g ~|~x_m > \tau}}^2.
    \end{equation}
    
    In contrast, if we split a new root node $\node_0$ on $m$ at the same threshold and call this split $s'$, we can run through a similar set of calculations to get
    \begin{equation} \label{eq:disentanglement_imp_dec_bigger}
    \Delta(s',\node_0,r) = \pi_2(x_m \leq \tau)\pi_2(x_m > \tau) \paren*{\E\braces*{f_2 - g ~|~x_m \leq \tau} - \E\braces*{f_2 - g ~|~x_m > \tau}}^2.
    \end{equation}
    Comparing \eqref{eq:disentanglement_imp_dec_smaller} and \eqref{eq:disentanglement_imp_dec_bigger}, we see that
    \begin{equation*}
        \Delta(s,\node, r^{(-1)}) = \pi_1(\node')\Delta(s',\node_0,r),
    \end{equation*}
    and as such, split $s'$ will be chosen in favor of $s$.
\end{proof}

\subsection{CART as a local orthogonal greedy procedure}

In this section, we build on recent work which shows that CART can be thought of as a ``local orthogonal greedy procedure''~\cite{klusowski2021universal}.
To see this, consider a tree model $\hat f$, and a leaf node $\node$ in the tree.
Given a potential split $s$ of $\node$ into children $\node_L$ and $\node_R$, we may associate the normalized decision stump
% \textit{Step 1: Feature engineering}. 
% Given a working tree model $\hat{f}$, we split a node $\mathfrak{t}$ according to some criteria (e.g. impurity decrease for CART). 
% This split $s$, we then learn the binary feature for each sample $\bx^{(i)}$ via the following function: 
\begin{equation} \label{eq:decision_stump}
\psi_{\node,s}(\bx) = \frac{N(\mathfrak{t}_{R})\mathbf{1}\{\bx \in \mathfrak{t}_{L}\} - N(\mathfrak{t}_{L})\{\bx \in \mathfrak{t}_{R}\}}{\sqrt{N(\node)N(\mathfrak{t}_{L})N(\mathfrak{t}_{R})}},
\end{equation}
% where $\node_L$ and $\node_R$ denote the left and right children of $\node$ respectively.
% This is a tri-valued function that is positive on the left child, negative on the right child, and zero everywhere else.
where $N(-)$ is used to denote the number of samples in a given node.
We use $\bPsi_{\node,s}$ to denote the vector in $\R^n$ comprising its values on the training set, noticing that it has unit norm.
If $\node$ is an interior node, then there is already a designated split $s(\node)$, and we drop the second part of the subscript.
It is easy to see that the collection $\braces*{\bPsi_\node}_{\node \in \hat f}$ is orthogonal to each other, and also to all decision stumps associated to potential splits.
This gives the second equality in the following chain
\begin{equation} \label{eq:impurity_dec_as_squared_dot_prod}
    \hat \Delta(s,\node) = \paren{\by^T \bPsi_{\node,s}}^2 = \paren{\br^T \bPsi_{\node,s}}^2,
\end{equation}
with the first being a straightforward calculation.
% In other words, the weighted impurity decrease is precisely the 
% Since $\norm{\bPsi_{\node,s}}_2^2 = 1$, this is equivalent to the squared Euclidean norm of the projected the response vector.
As such, the CART splitting condition is equivalent to selecting a feature vector from an admissible set that best reduces the residual variance.

Concatenating the decision stumps together yields a feature map $\Psi\colon \R^d \to \R^p$, and we let $\bPsi$ denote the $n$ by $m$ transformed data matrix.
Let $\hat{\bbeta}$ denote the solution to the least squares problem
\begin{equation} \label{eq:least_squares_CART}
     \min_{\bbeta} ~ \norm*{\bPsi\bbeta - \by}_2^2.
\end{equation}
\cite{klusowski2021universal} was able to show (see Lemma 3.2 therein) that we have functional equality
\begin{equation} \label{eq:CART_as_lin_reg}
    \hat f(\bx) = \hat{\bbeta}^T \Psi(\bx).
\end{equation}

\subsection{Modifications for \method}
\label{subsec:FIGS_linear_supp}

With a collection of trees $\tree_1,\ldots,\tree_K$, we may still associate a normalized decision stump \eqref{eq:decision_stump} to every node, solve \eqref{eq:least_squares_CART} and then turn \eqref{eq:CART_as_lin_reg} into a definition for $\hat f$.
To see what kind of function $\hat f$ is, let $J_1,\ldots,J_K$ denote the blocks of decision stump feature indices belonging to different trees.
For each block $k$, we have the local optimality condition
\begin{equation}
     \hat\bbeta_{J_k} = \argmin_{\bbeta'} ~ \norm*{\bPsi_{J_K}\bbeta' - \br^{(-k)}}_2^2.
\end{equation}
where
\begin{equation*}
    \br^{(-k)} = \by - \bPsi_{-J_k}\hat \bbeta_{-J_k}.
\end{equation*}
Note that here and in the rest of this section, subscripts on vectors will refer to restrictions or exclusions of subsets of coordinates.
Furthermore, our use of this notation for the residual is not coincidental.
By invoking \eqref{eq:CART_as_lin_reg} for a single tree, we see that the function $\bx \mapsto \hat{\bbeta}_{J_k}^T \Psi_{J_k}(\bx)$ is constant on the leaves of $\tree_k$, and on each leaf predicts the mean of $r^{(-k)}$ over the samples in that leaf.
As such, $\hat f(\bx) \coloneqq \hat{\bbeta}^T \Psi(\bx)$ is a tree-sum model satisfying \eqref{eq:best_fit_property} in \cref{sec:theory}.
Indeed, since it is easy to see that it is best-fit.
If the columns of $\bPsi$ are linearly independent, then it is the unique best-fit tree-sum model.
We will use this interpretation of the tree-sum model in the ensuing proof.

Meanwhile, a version of \eqref{eq:impurity_dec_as_squared_dot_prod} continues to hold, with
$$
\hat \Delta(s,\node,r^{(-k)}) = \paren{\br^{(-k)T}\bPsi_{\node,s}} ^2.
$$
On the other hand, because the features are not orthogonal, this no longer corresponds to the reduction in residual variance.

\subsection{Helper lemmas on linear regression}

We consider the case of possibly under-determined least squares, i.e. the problem
\begin{equation} \label{eq:least_squares}
     \min_{\btheta} ~ \norm*{\bX\btheta - \by}_2^2
\end{equation}
where we allow for the possibility that $\bX$ does not have linearly independent columns.
When this is indeed the case, there will be multiple solutions to \eqref{eq:least_squares}, but there is a unique element $\hat{\btheta}$ of the solution set that has minimum norm.
In fact, this is given by the formula
$$
\hat{\btheta} = \bX^{\dagger}\by,
$$
where $\bX^\dagger$ denotes the Moore-Penrose pseudo-inverse of $\bX$.

We extend the definition of leverage scores to this case by defining the $i$-th leverage score $h_i$ to be the $i$-th diagonal entry of the matrix $\bH \coloneqq \bX\bX^\dagger$.
Note that the vector of predicted values is given by we have
$$
\hat\by = \bX\hat\btheta = \bX\bX^{\dagger}\by = \bH\by,
$$
so that this coincides with the definition of leverage scores in the linearly independent case.

In what follows, we will work extensively with leave-one-out (LOO) perturbations of the sample and the resulting estimators.
We shall use $\bX^{(-i)}$ to denote the data matrix with the $i$-th data point removed, and $\hat \btheta^{(-i)}$ to denote the solution to \eqref{eq:least_squares} with $\bX$ replaced with $\bX^{(-i)}$.
We have the following two generalizations of standard formulas in the full rank setting.

\begin{lemma}[Leave-one-out estimated coefficients] \label{lem:LOO_coefficients}
    The LOO estimated coefficients satisfy
    \begin{equation*}
        \bx_i^{T}\paren*{\hat\btheta - \hat\btheta^{(-i)}} = \frac{h_i\hat e_i}{1-h_i}
    \end{equation*}
    where $\hat e_i = y_i - \bx_i^T\hat\btheta$ is the residual from the full model.
\end{lemma}

\begin{proof}
    Note that we may write $\bX^\dagger = \paren*{\bX^T\bX}^\dagger\bX^T$.
    We may then follow the proof of the usual identity but substituting \eqref{eq:sherman_morrison} in lieu of the regular Sherman-Morrison formula.
\end{proof}

\begin{lemma}[Sherman-Morrison]
    Let $\bX$ be any matrix. Then
    \begin{equation} \label{eq:sherman_morrison}
        \paren*{\bX^{(-i)T}\bX^{(-i)}}^\dagger = \paren*{\bX^T\bX}^{\dagger} + \frac{\paren*{\bX^T\bX}^{\dagger}\bx_i\bx_i^T\paren*{\bX^T\bX}^{\dagger}}{1-h_i}.
    \end{equation}
\end{lemma}

\begin{proof}
    We apply Theorem 3 in \cite{meyer1973generalized} to $A = \bX^T\bX$, $c = \bx_i$ and $d = - \bx_i$, noting that the necessary conditions are fulfilled.
\end{proof}

\begin{theorem}[Generalization error for linear regression] \label{thm:generalization_lin_reg}
    Consider a linear regression model
    $$
    y = \btheta^T\bx + \epsilon + \eta
    $$
    where $\sup_\bx \paren*{\btheta^T\bx}^2 \leq B^2$, $\epsilon$ and $\eta$ are independent, $\E\braces*{\epsilon~|~\bx} = \E\braces*{\eta~|~\bx} = 0$, $\E\braces*{\epsilon^2~|~\bx} = \sigma_\epsilon^2$, and $\E\braces*{\eta^2} = \sigma_\eta^2$.
    Given a training set $\data$, and a query point $\bx$, let $\hat\btheta_n$ be the estimated regression vector.
    %, and let $\hat{f}_n$ be the predictor that, given a query point $\bx$, outputs $\btheta_n^T\bx$, where $\bX$ is the training data matrix vertically concatenated with $\bx$.
    There is an event $\mathcal{E}$ of probability at most $2p/n$ over which we have
    \begin{equation}
        \E_{\data,\bx}\braces*{\paren*{\bx^T\paren*{\hat\btheta_{n} - \btheta}}^2\indicator\braces*{\mathcal E ^c}}
        \leq 2\paren*{\frac{p\sigma_\epsilon^2}{n+1} + 2\sigma_\eta^2}.
    \end{equation}
\end{theorem}

\begin{proof}
    Let $\data$ denote the training set. Let $\mathcal{E}$ be the event on which $\bx^T\paren*{\bX^T\bX}^{\dagger}\bx \leq \frac{1}{2}$. 
    This quantity is the leverage score for $\bx$, so that
    $$
    \E\braces*{\bx^T\paren*{\bX^T\bX}^{\dagger}\bx} \leq \frac{p}{n+1}
    $$
    by exchangeability of $\bx$ with the data points in $\data$.
    We may then apply Markov's inequality to get
    $$
    \P\braces*{\mathcal E} \leq \frac{2p}{n+1}.
    $$
    
    Again using exchangeability, we may write
    \begin{align} \label{eq:risk_decomposition}
        \E_{\data,\bx}\braces*{\paren*{\bx^T\paren*{\hat{\btheta}_n - \btheta}}^2\indicator\braces*{\mathcal{E}^c}} 
        = \frac{1}{n+1} \sum_{i=0}^n\E_{\data[n+1]} \braces*{\paren*{\bx_i^T\paren*{\hat{\btheta}_{n+1}^{(-i)} - \btheta}}^2\indicator\braces*{\mathcal{E}_i^c}},
    \end{align}
    where $\data[n+1]$ is the augmentation of $\data$ with the query point $\bx_0 = \bx$ and response $y_0$, $\hat{\btheta}_{n+1}$ is the regression vector learnt from $\data[n+1]$, and for each $i$, $\hat{\btheta}_{n+1}^{(-i)}$ that from $\data[n+1]\backslash \braces*{\paren*{\bx_i,y_i}}$.

    To bound this, we first rewrite the prediction error for the full model as
    \begin{align} \label{eq:full_model_pred_error}
        \bx_i^T\paren*{\hat\btheta_{n+1} -\btheta} 
        & = \bx_i^T\bX^\dagger \by - \bx_i^T\btheta \nonumber \\
        & = \bx_i^T\bX^\dagger \paren*{\bX\btheta + \beps + \beeta} - \bx_i^T\btheta \nonumber \\
        & = \bx_i^T\bX^\dagger\paren*{\beps + \beeta},
    \end{align}
    where the last equality follows because $\bx_i$ lies in the column space of $\bX^\dagger\bX$.
    Next, we may decompose that for the LOO model as
    \begin{equation} \label{eq:LOO_model_pred_error}
        \bx_i^T\paren*{\hat{\btheta}_{n+1}^{(-i)} - \btheta} 
        = \bx_i^T\paren*{\hat{\btheta}_{n+1}^{(-i)} - \hat\btheta_{n+1}} + \bx_i^T\paren*{\hat\btheta_{n+1} - \btheta}.
    \end{equation}
    We expand the first term using Lemma \ref{lem:LOO_coefficients} to get
    \begin{align} \label{eq:full_and_LOO_diff}
        \bx_i^T\paren*{\hat{\btheta}_{n+1}^{(-i)} - \hat\btheta_{n+1}}
        & = \frac{h_i}{1-h_i}\paren*{\bx_i^T\hat\btheta_{n+1} - y_i} \nonumber \\
        & = \frac{h_i}{1-h_i}\paren*{\bx_i^T\paren*{\hat\btheta_{n+1} - \btheta} - \epsilon_i - \eta_i}.
    \end{align}
    We plug \eqref{eq:full_and_LOO_diff} into \eqref{eq:LOO_model_pred_error} and then \eqref{eq:full_model_pred_error} into the resulting equation to get
    \begin{align*}
        \bx_i^T\paren*{\hat{\btheta}_{n+1}^{(-i)} - \btheta} 
        & = \frac{h_i}{1-h_i}\paren*{\bx_i^T\paren*{\hat\btheta_{n+1} - \btheta} - \epsilon_i - \eta_i} + \bx_i^T\paren*{\hat\btheta_{n+1} - \btheta} \\
        & = \frac{1}{1-h_i} \paren*{\bx_i^T\paren*{\hat\btheta_{n+1} - \btheta}} - \frac{h_i}{1-h_i}\paren*{\epsilon_i + \eta_i} \\
        & = \frac{1}{1-h_i} \bx_i^T\bX^\dagger\paren*{\beps + \beeta} - \frac{h_i}{1-h_i}\paren*{\epsilon_i + \eta_i}.
    \end{align*}
    Taking expectations and using the independence of $\beps$ and $\beeta$, we get
    \begin{align*}
        \E \braces*{\paren*{\bx_i^T\paren*{\hat{\btheta}_{n+1}^{(-i)} - \btheta}}^2\indicator\braces*{\mathcal{E}_i^c}} 
        & = \E\braces*{\paren*{\frac{\bx_i^T\bX^\dagger\beps - h_i\epsilon_i}{1-h_i}}^2\indicator\braces*{\mathcal{E}_i^c}} 
        + \E\braces*{\paren*{\frac{\bx_i^T\bX^\dagger\beeta - h_i\eta_i}{1-h_i}}^2\indicator\braces*{\mathcal{E}_i^c}} \nonumber\\
        & \leq \E\braces*{\paren*{\frac{\bx_i^T\bX^\dagger\beps - h_i\epsilon_i}{1-h_i\wedge 1/2}}^2} 
        + \E\braces*{\paren*{\frac{\bx_i^T\bX^\dagger\beeta - h_i\eta_i}{1-h_i \wedge 1/2}}^2}.
    \end{align*}
    Summing up the first term over all indices, and then taking an inner expectation with respect to $\beps$, we get
    \begin{align}  \label{eq:sq_error_first_term}
        \frac{1}{n+1}\sum_{i=0}^n \E\braces*{\paren*{\frac{\bx_i^T\bX^\dagger\beps - h_i\epsilon_i}{1-h_i\wedge 1/2}}^2} 
        & = \frac{1}{n+1}\E\braces*{\norm*{\paren{1-\diag\paren*{\bH}\wedge 1/2}^{-1}\paren*{\bH - \diag\paren*{\bH}}\beps}_2^2} \nonumber\\
        & = \frac{\sigma_\epsilon^2}{n+1}\E\braces*{\trace\paren*{\bW\bW^T}}.
    \end{align}
    where
    $$
    \bW = \paren{1-\diag\paren*{\bH}\wedge 1/2}^{-1}\paren*{\bH - \diag\paren*{\bH}}.
    $$
    Since $\bH$ is idempotent, we get
    $$
    \paren*{\bH - \diag\paren*{\bH}}^2 = \bH - \bH\diag\paren*{\bH} - \diag\paren*{\bH}\bH + \diag\paren*{\bH}^2.
    $$
    The $i$-th summand in the trace therefore satisfies
    \begin{align*}
        \paren*{\bW\bW^T}_{ii} & = \frac{h_i - 2h_i^2 + h_i^2}{\paren*{1 - h_i\wedge 1/2}^2} \\
        & \leq \frac{h_i}{1 - h_i\wedge 1/2} \\
        & \leq 2h_i.
    \end{align*}
    Summing these up, we therefore continue \eqref{eq:sq_error_first_term} to get
    \begin{equation} \label{eq:sq_err_first_term_final}
        \frac{\sigma_\epsilon^2}{n+1}\E\braces*{\trace\paren*{\bW\bW^T}} \leq \frac{2\sigma_\epsilon^2}{n+1}\E\braces*{\trace\paren*{\bH}} \leq \frac{2p\sigma_\epsilon^2}{n+1}.
    \end{equation}
    
    Next, for any $\bx$, we slightly abuse notation, and denote $\sigma_\eta^2(\bx) = \E\braces*{\eta^2~|~\bx}$.
    By a similar calculation, we get
    $$
    \frac{1}{n+1}\sum_{i=0}^n \E\braces*{\paren*{\frac{\bx_i^T\bX^\dagger\beeta - h_i\eta}{1-h_i\wedge 1/2}}^2} 
    = \frac{1}{n+1}\E\braces*{\trace\paren*{\bW\bSigma\bW^T}},
    $$
    where $\bSigma$ is a diagonal matrix with entries given by $\bSigma_{ii} = \sigma_\eta^2(\bx_i)$ for each $i$.
    We compute
    \begin{align*}
        \paren*{\bW\bSigma\bW^T}_{ii} 
        = \frac{\sum_{j \neq i} \bH_{ij}^2\sigma_\eta(\bx_j)^2}{\paren*{1-h_i \wedge 1/2}^2} 
        \leq 4\sum_{j=0}^n \bH_{ij}^2\sigma_\eta(\bx_j)^2 
        = 4\paren*{\bH\bSigma\bH^T}_{ii}.
    \end{align*}
    This implies that
    \begin{align} \label{eq:sq_err_second_term_final}
        \frac{1}{n+1}\E\braces*{\trace\paren*{\bW\bSigma\bW^T}} 
        & \leq \frac{4}{n+1}\E\braces*{\trace\paren*{\bH\bSigma\bH^T}} \nonumber\\
        & \leq \frac{4}{n+1}\E\braces*{\trace\paren*{\bSigma}} \nonumber\\
        & = 4\sigma_\eta^2.
    \end{align}
    Applying \eqref{eq:sq_err_first_term_final} and \eqref{eq:sq_err_second_term_final} into \eqref{eq:risk_decomposition} completes the proof.
\end{proof}

\begin{remark}
    Note that while we have bounded the probability of $\mathcal{E}$ by $\frac{2p}{n}$, it could be much smaller in value.
    If $\Psi$ is constructed out of a single tree, then $\mathcal{E}$ holds if and only if the test point lands in a leaf containing no training points.
    \cite{tan2021cautionary} shows that the probability of this event decays exponentially in $n$.
\end{remark}
